# Supplementary material for: DPC: Unsupervised Deep Point Correspondence via Cross and Self Construction
Source: arXiv:2110.08636 source file (2021-10-16)

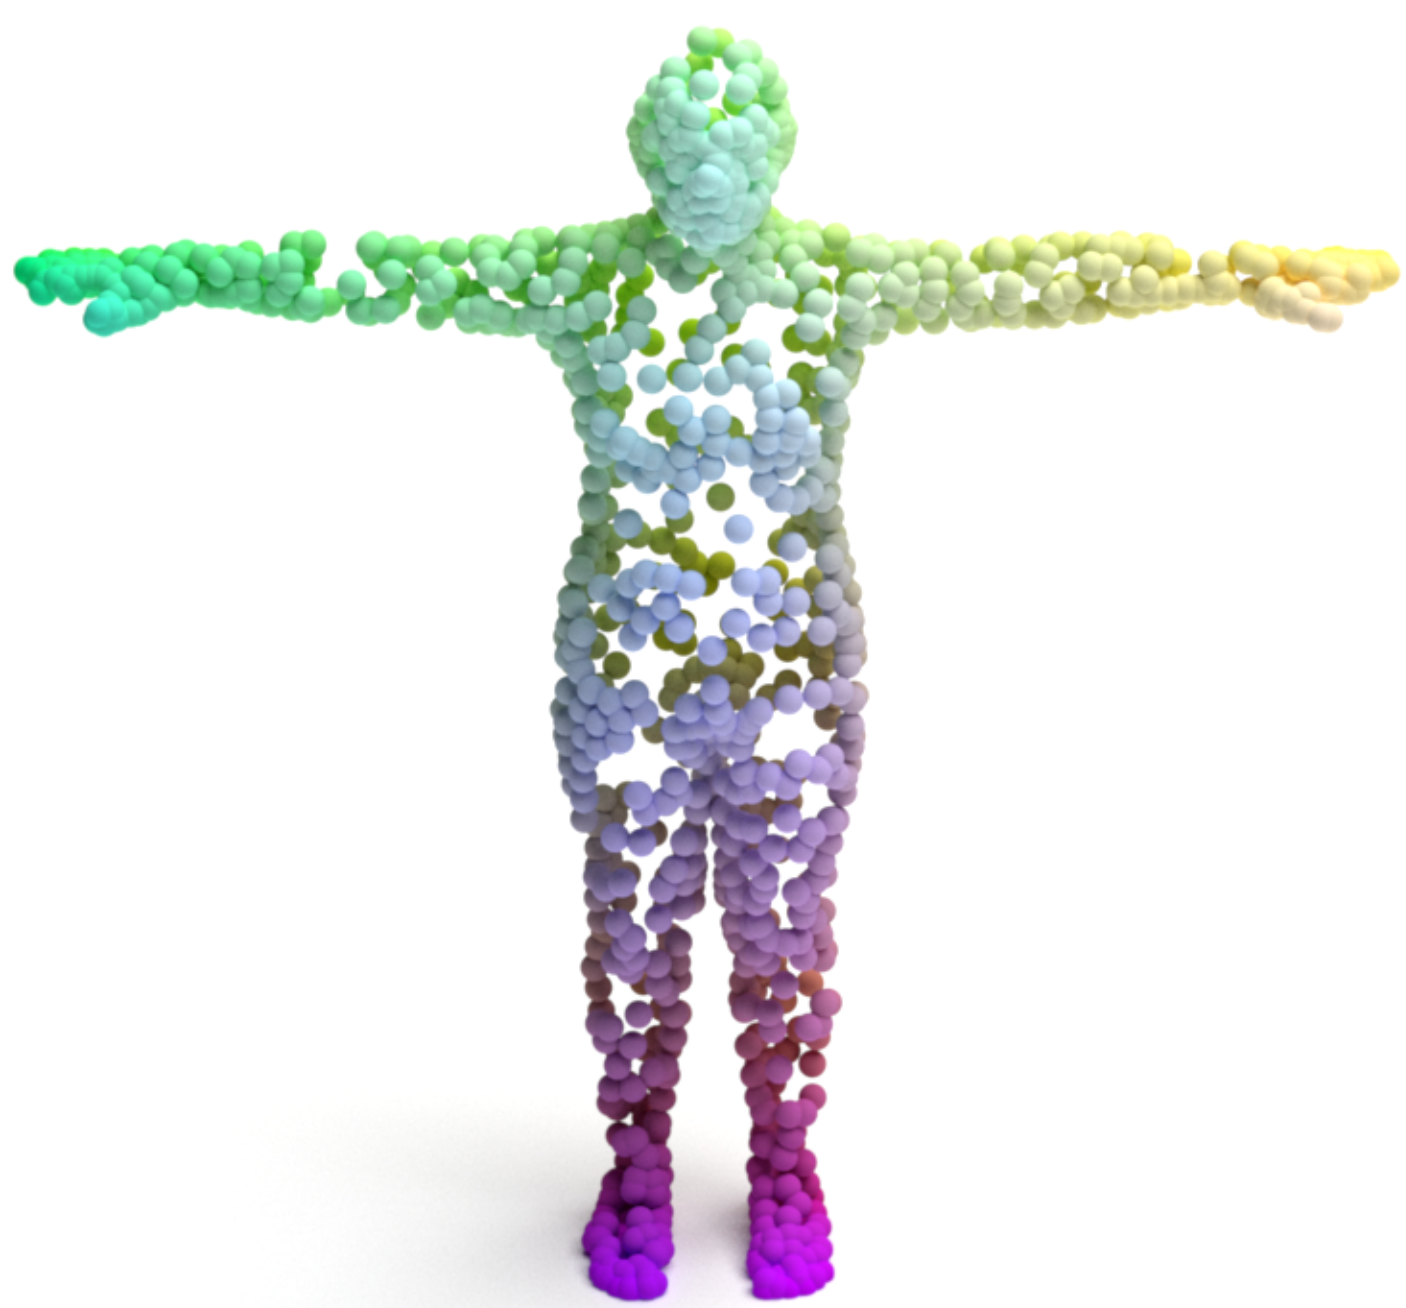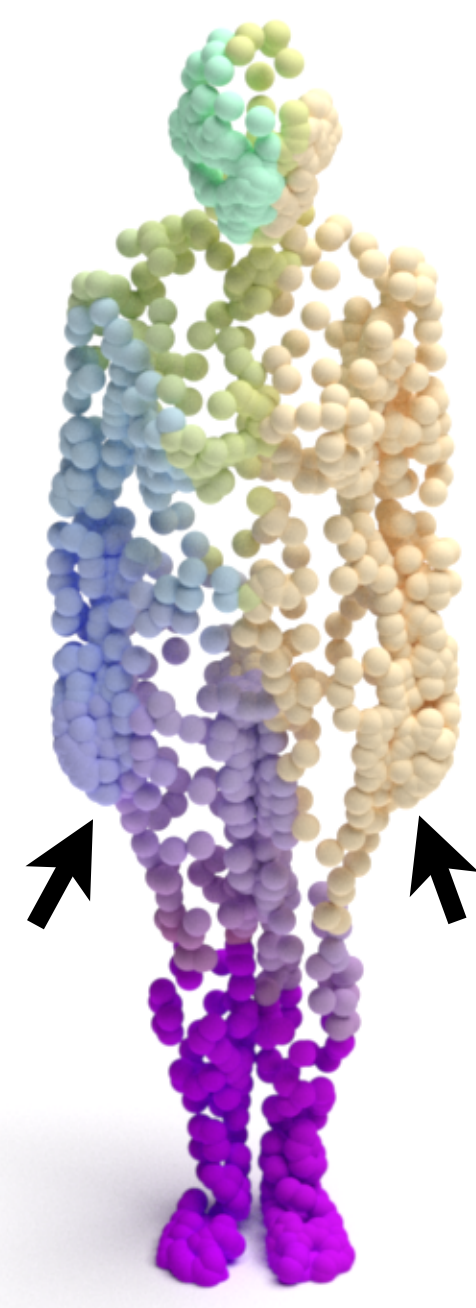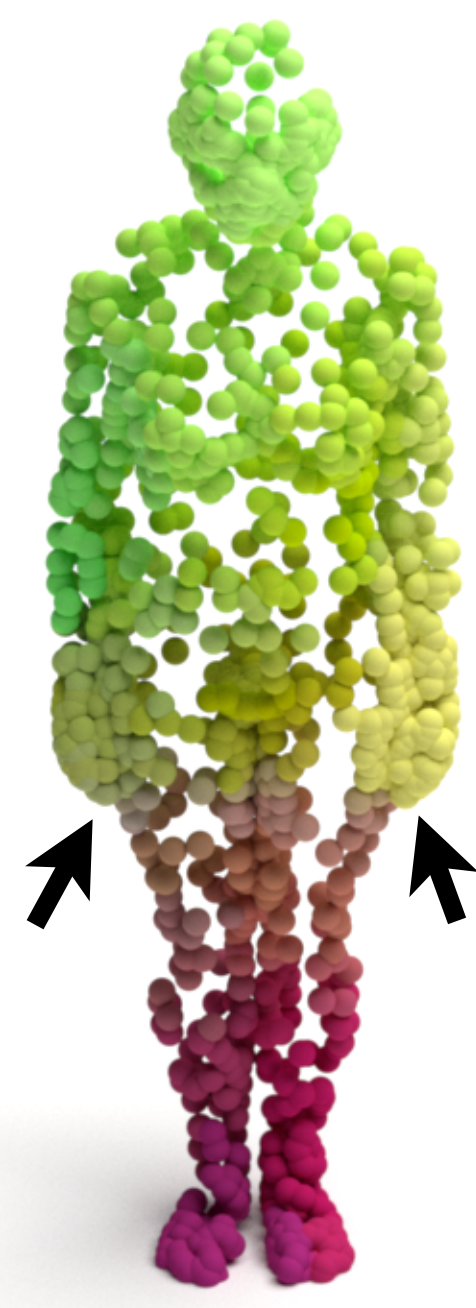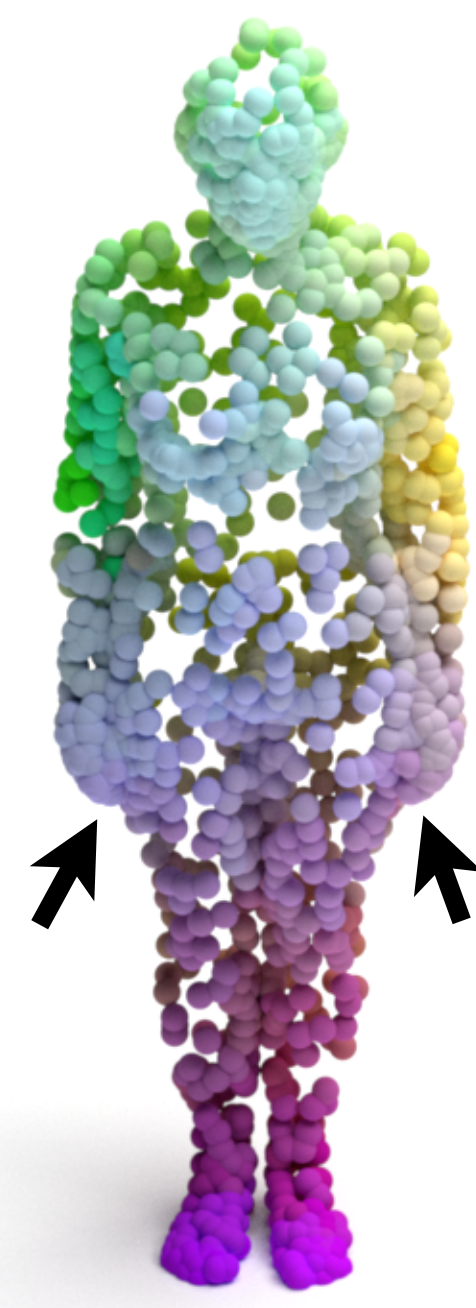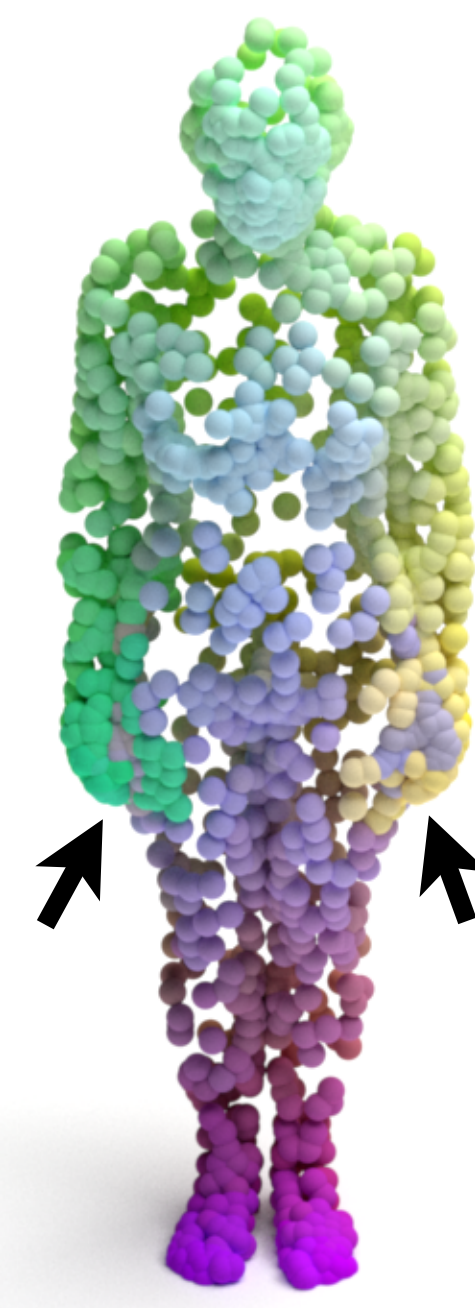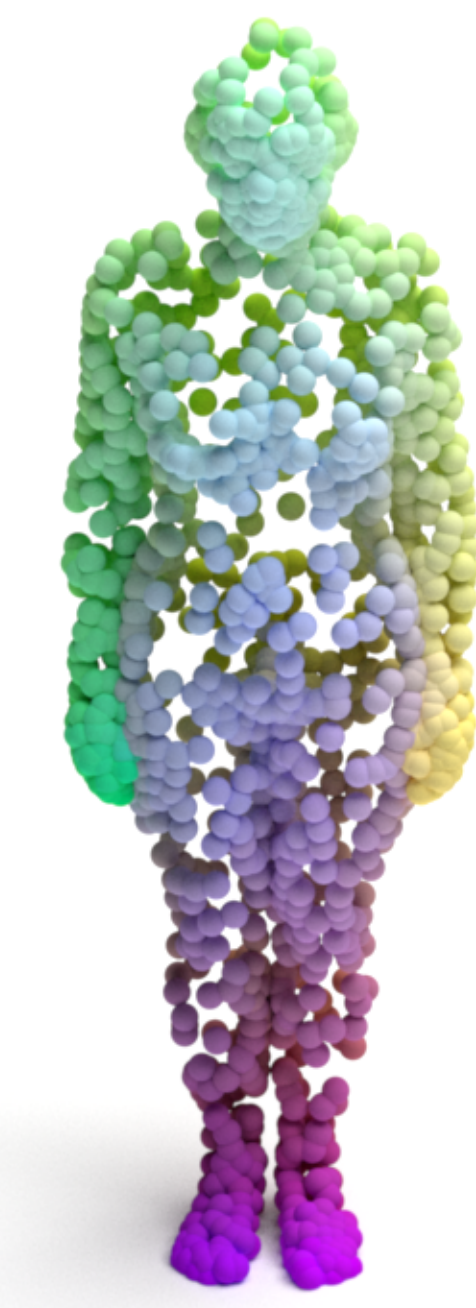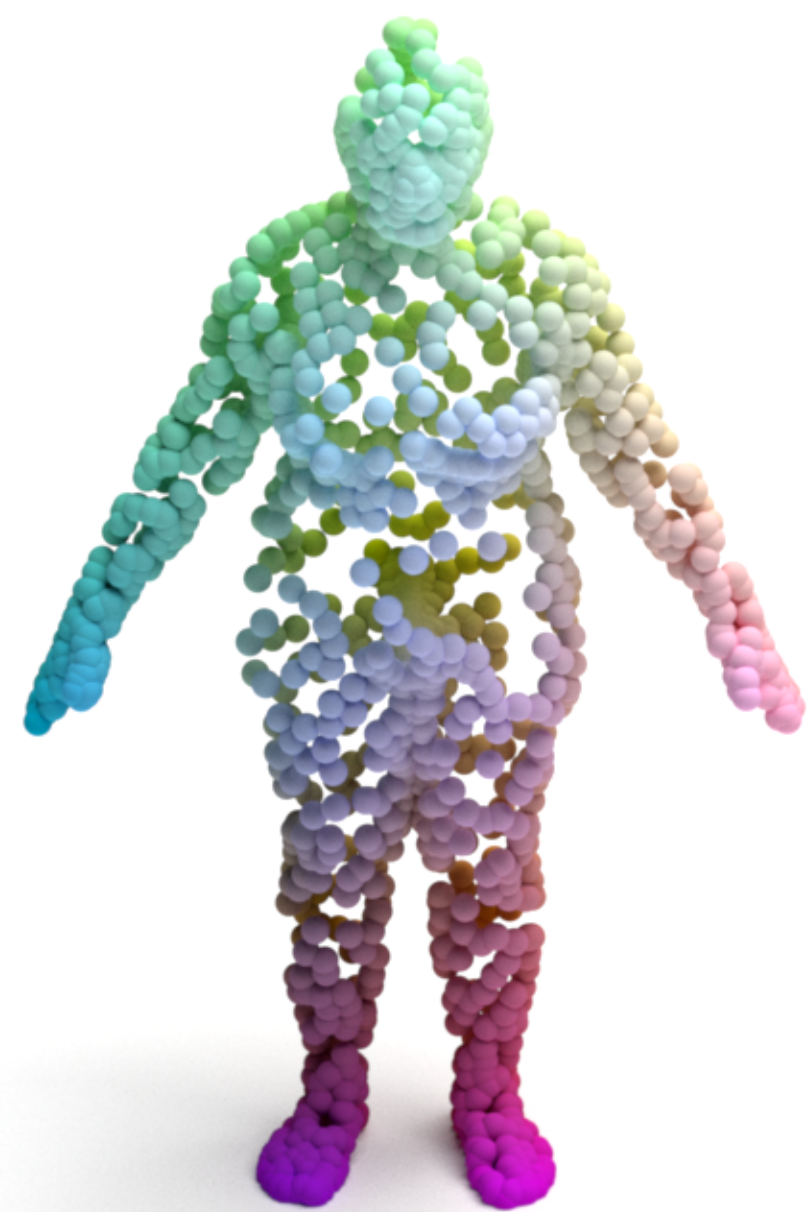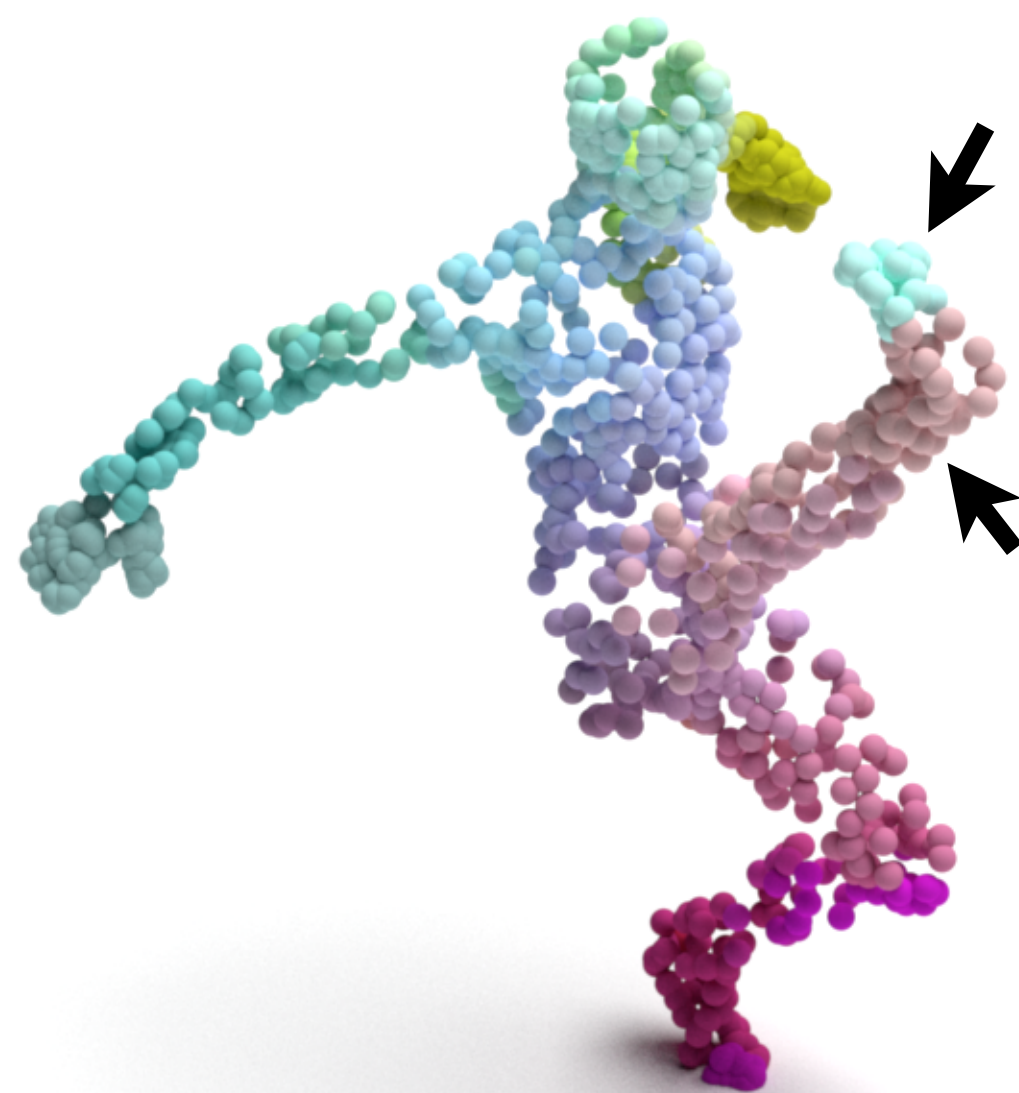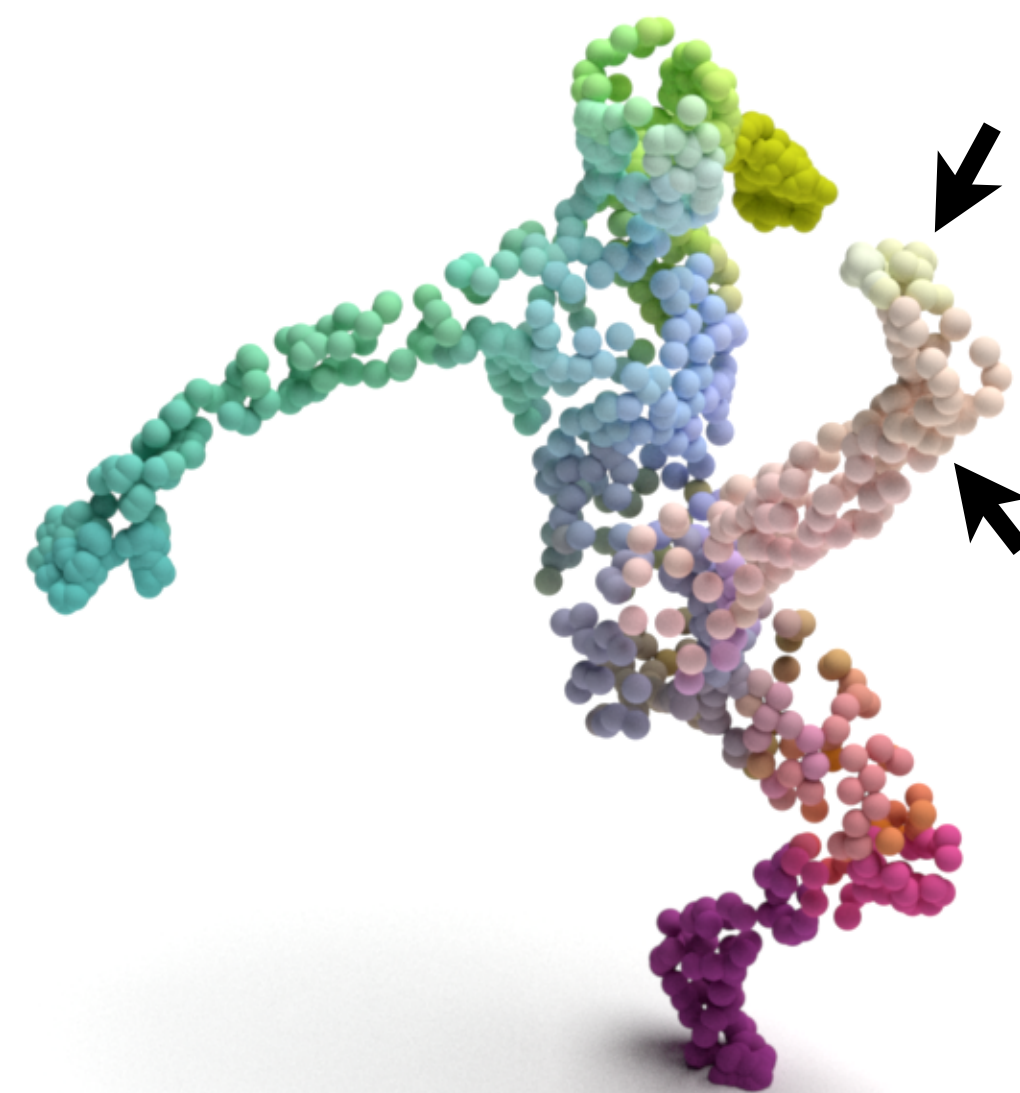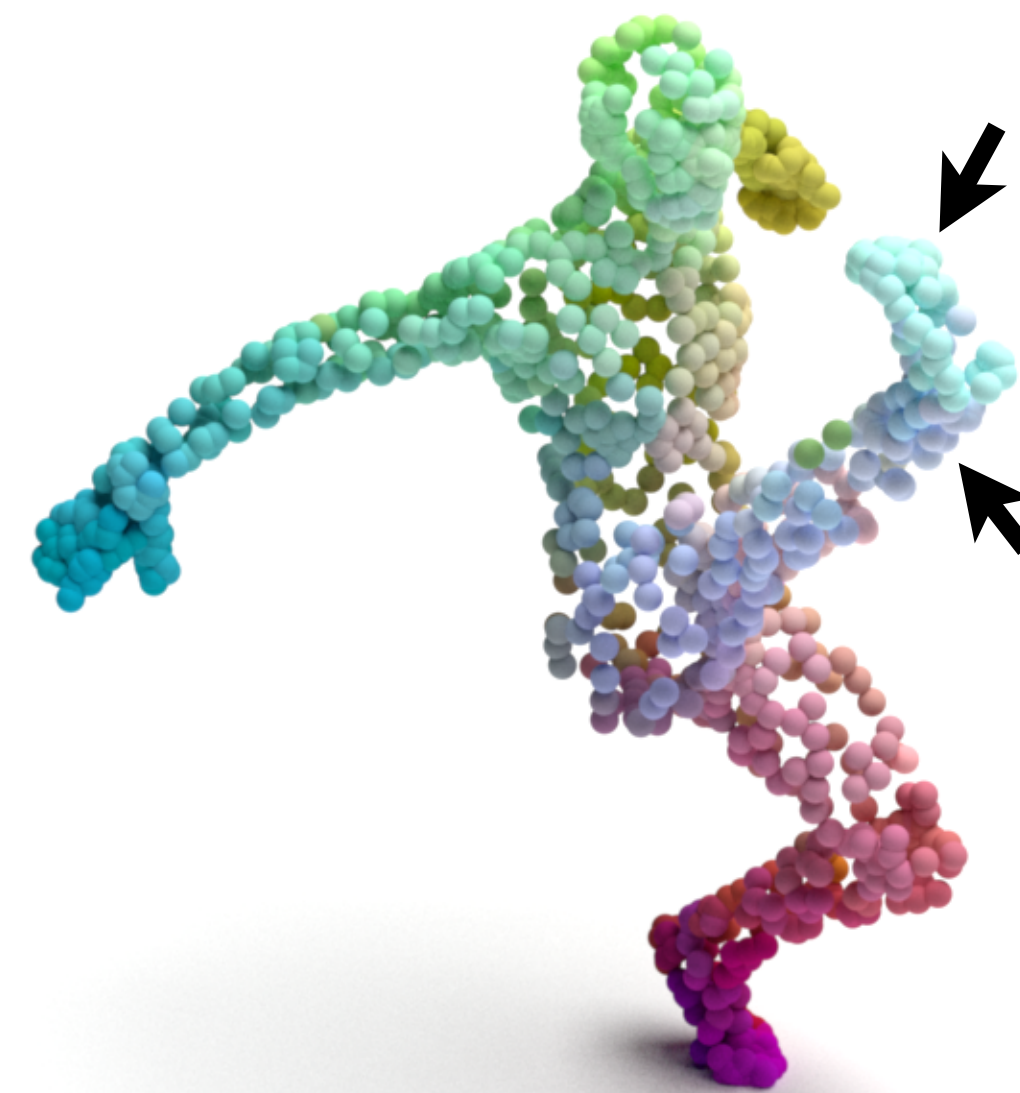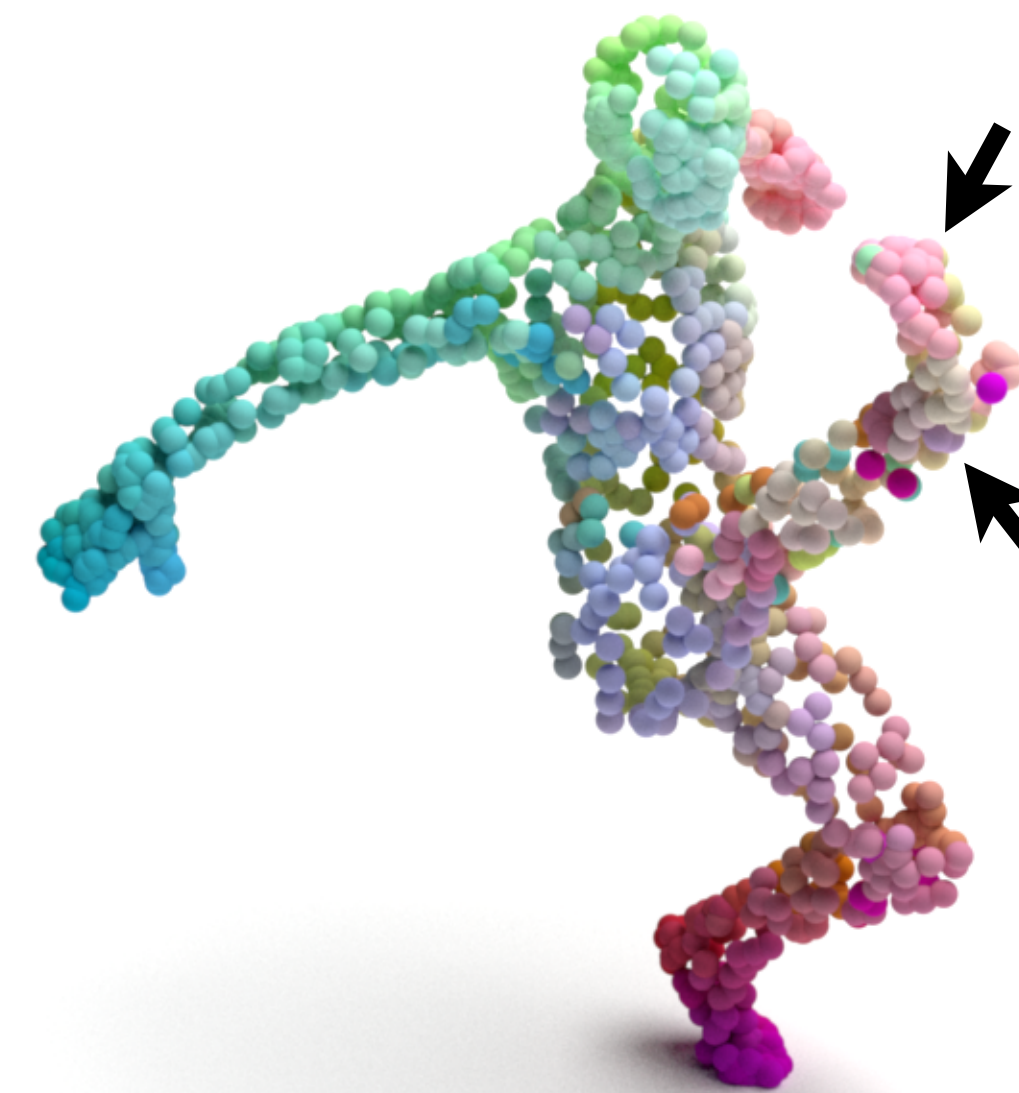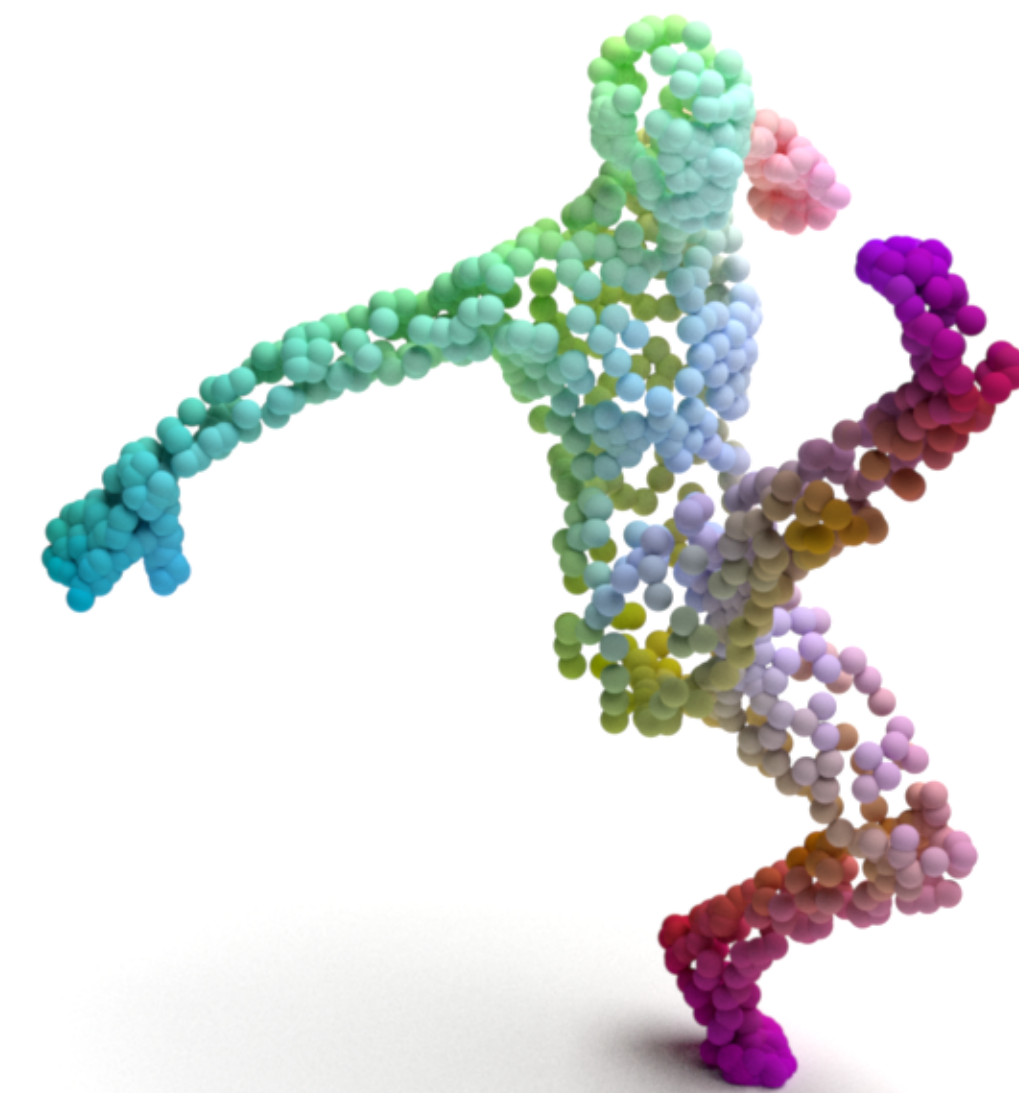

Supplement: Supplementary file 1 [file failure_cases.pdf]
