# Supplementary material for: DPC: Unsupervised Deep Point Correspondence via Cross and Self Construction
Source: arXiv:2110.08636 source file (2021-10-16)
Supplement: Supplementary file 2 [file resolution_robustness.pdf]

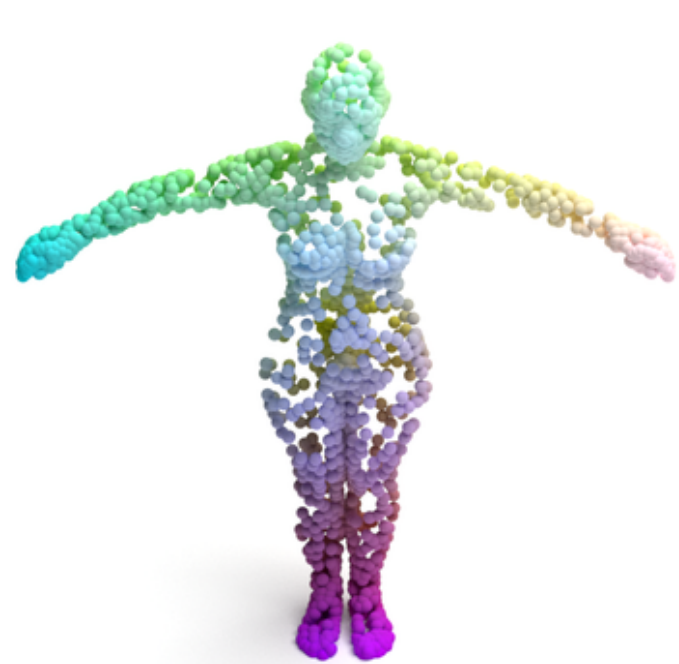

Target 1024

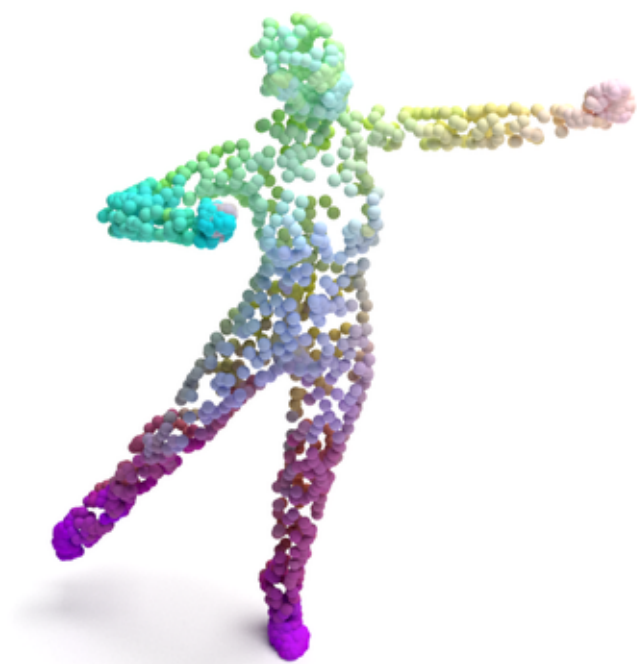

Source 1024

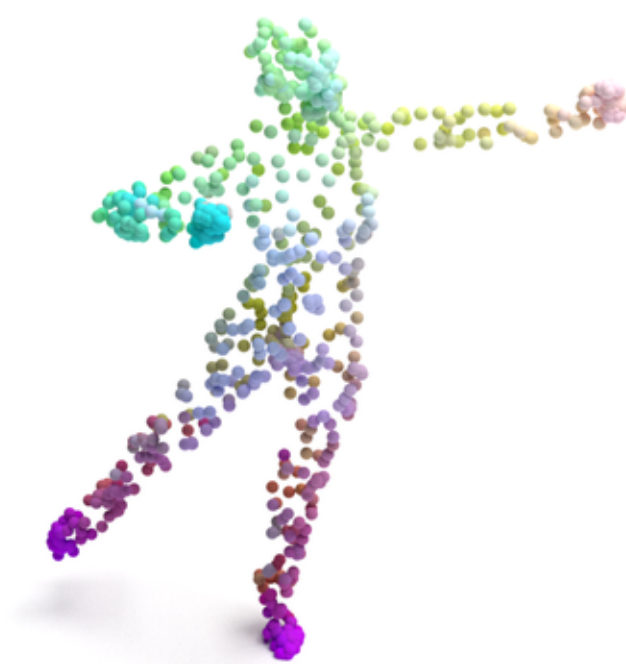

Source 512

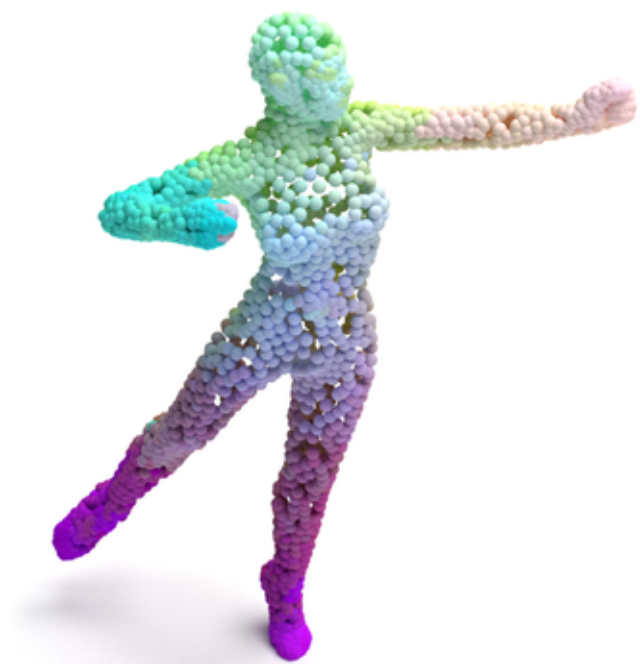

Source 4096
