# Supplementary material for: DPC: Unsupervised Deep Point Correspondence via Cross and Self Construction
Source: arXiv:2110.08636 source file (2021-10-16)
Supplement: Supplementary file 3 [file train_size_pdf.tex]

\begin{figure}[tb!]
\begin{center}
\includegraphics[width=\columnwidth]{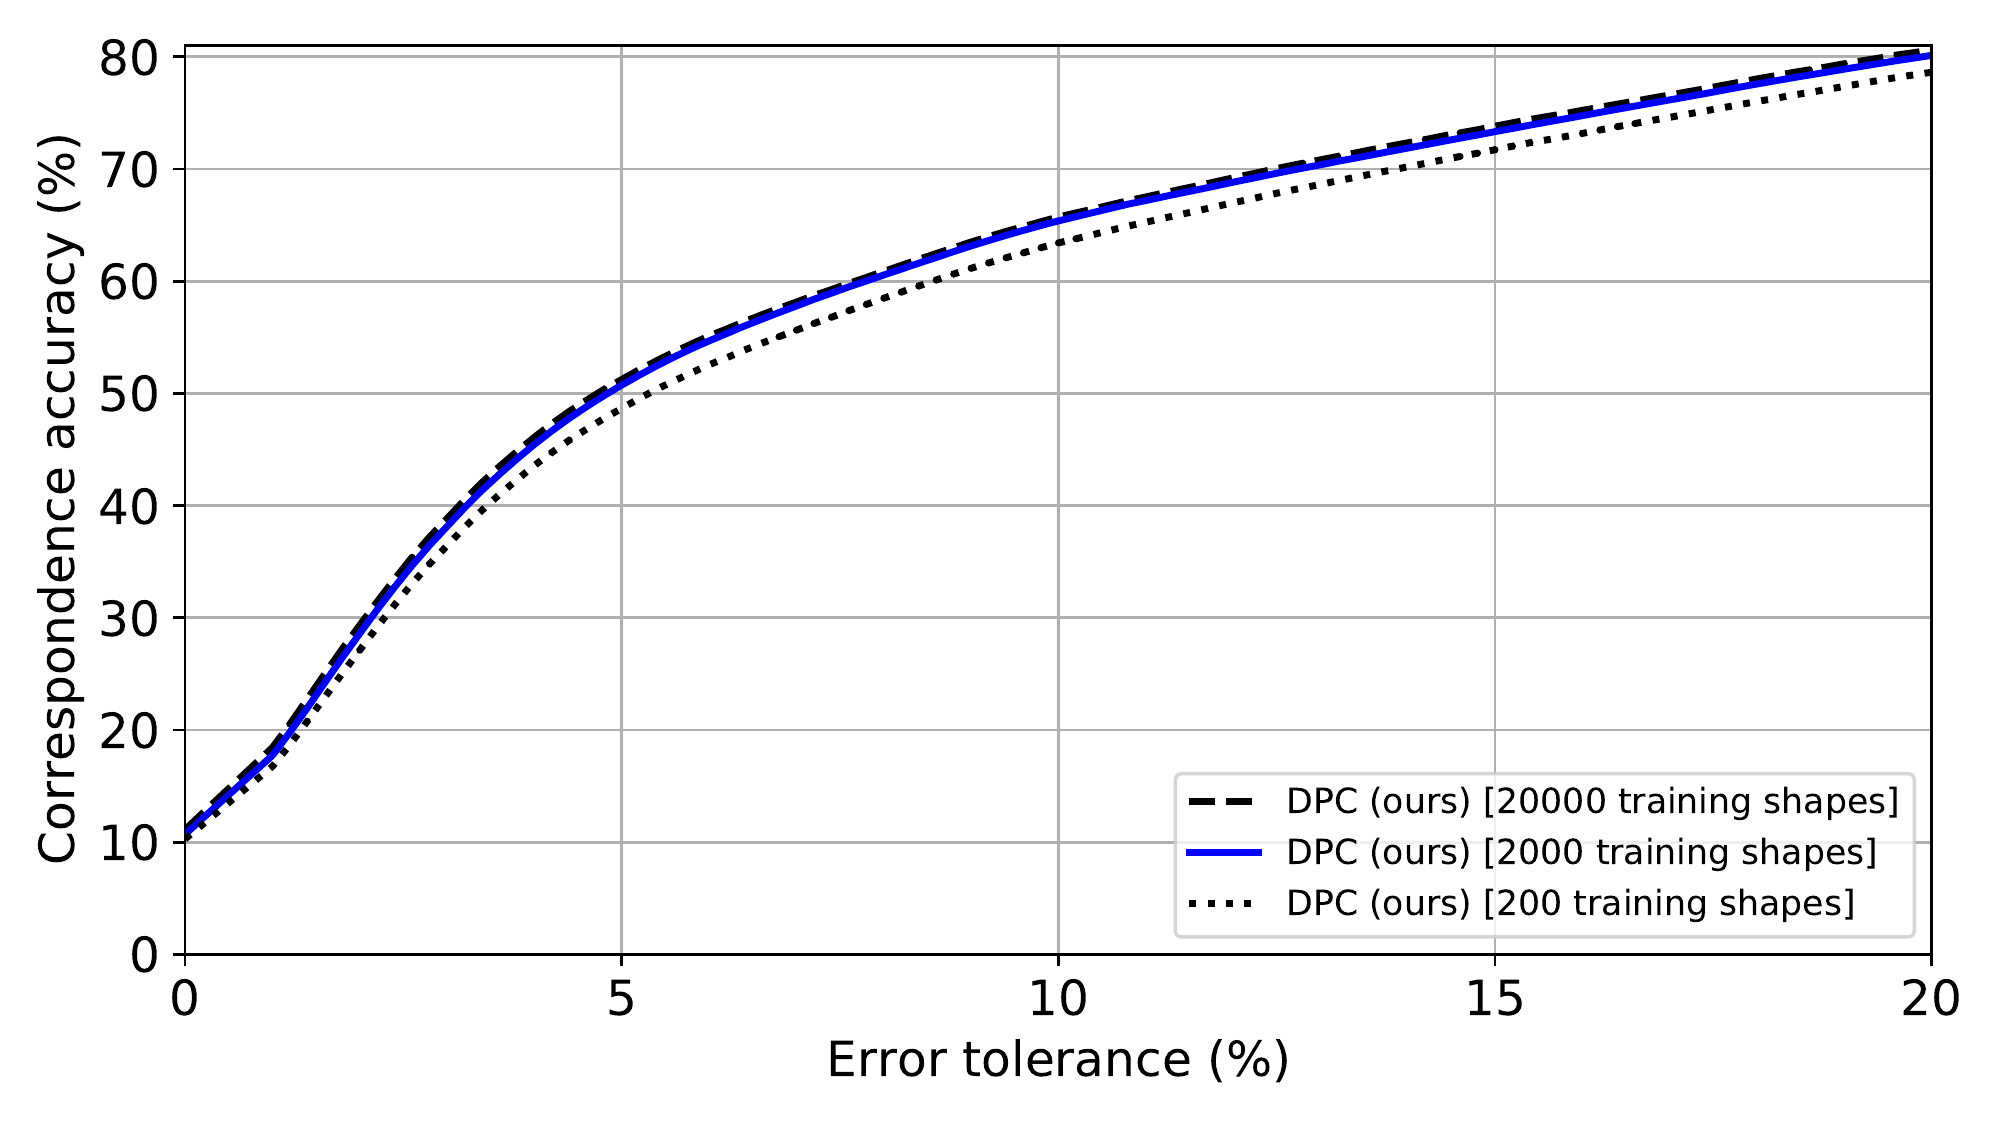}
\caption{{\bfseries Correspondence accuracy for difference train set size.} DPC was trained on the SURREAL dataset with a different number of training examples and evaluated on SHREC'19 test pairs. Using only 2000 shapes is sufficient for reaching the model's potential performance.}
\label{fig:train_size_supp}
\end{center}
\end{figure}
